# Supplementary material for: OPDMulti: Openable Part Detection for Multiple Objects
Source: arXiv:2303.14087 source file (2023-03-24)
Supplement: Supplementary file 1 [file 01-implementation-details.tex]

\section{Additional implementation details}
\label{sec:supp:implementation}

\mypara{Network structure for multiple object pose prediction} 
For \opdrcnnop and \opdformerp, we predict object pose for each part separately. Similar to the motion parameters, we add MLP to the box head for \opdnet and the mask module for OPDFormer. \todo{Do we need a simple figure to illustrate this? Or, is it too simple? Maybe we don't need to include this section in the supplement}
