# Supplementary material for: OPDMulti: Openable Part Detection for Multiple Objects
Source: arXiv:2303.14087 source file (2023-03-24)
Supplement: Supplementary file 2 [file tab-results-meanstd-opdmulti.tex]

\begin{table}
\resizebox{\linewidth}{!}
{
\begin{tabular}{@{} l rrrr @{}}
\toprule
& & \multicolumn{3}{c}{Part-averaged mAP $\% \uparrow$} \\
\cmidrule(l{0pt}r{2pt}){2-5}
 Model & \partdet & +\mtype & +\mtype{}\axis & +\mtype{}\axis{}\orig \\
\midrule
\opdrcnnc~\cite{jiang2022opd} & 27.2\std{0.06} & 25.7\std{0.03} & 9.0\std{0.15} & 7.9\std{0.13} \\
\opdrcnno~\cite{jiang2022opd} & 20.5\std{0.67} & 18.5\std{0.84} & 4.1\std{0.09} & 0.7\std{0.03} \\
\opdrcnnop & 21.3\std{0.64} & 19.3\std{0.53} & 7.5\std{0.28} & 5.9\std{0.23} \\
% \cmidrule(l{0pt}r{2pt}){2-9}
\opdformerc & 30.0\std{1.02} & 28.6\std{0.99} & 13.0\std{0.55} & 12.0\std{0.49} \\
\opdformero & 29.4\std{0.56} & 27.7\std{0.60} & 5.3\std{0.15} & 1.7\std{0.09} \\
\opdformerp & \best{33.1\std{0.38}} & \best{31.9\std{0.35}} & \best{19.6\std{0.50}} & \best{16\std{0.25}} \\
\bottomrule
\end{tabular}
}
\caption{Comparison of \opdrcnn and \opdformerbaseline on validation set RGB input images for \ourdatamulti dataset with random seeds.}
\label{tab:results-OPDAll-val-meanstd-mini}
\end{table}
